# Supplementary material for: Efficient and Effective Algorithms for A Family of Influence Maximization Problems with A Matroid Constraint
Source: arXiv:2410.16603 source file (2024-10-22)
Supplement: Supplementary file 1 [file temp.tex]

\newpage
\section{Issues about \advim}

\yiqian{This is quite informal. We could just treat it as a whiteboard. After everything is figured out, I will remove it.}

\stitle{Revisiting Lemma 2}
In the following, we use the notations in~\cite{sun2023scalable}:
\begin{itemize}[topsep=2pt,itemsep=1pt,parsep=0pt,partopsep=0pt,leftmargin=11pt]
    \item $S$ is the original seed set; 
    \item $A$ is the set we chose;
    \item $P_L$ is an RR path (containing nodes and edges) starting from a node selected uniformly from $V\backslash S$ at random;
    \item $P^S_L$ is a `relevant' RR path, which is equal to $P_L$ if $P_L$ intersects with $S$, and $\emptyset$ otherwise;
    \item $n^-=|V|-|S|$;
    \item $\sigma^-(S)=\sigma(S)-|S|$;
    \item $VE(X)=X\backslash S$;
    \item $\Gamma(L, S)$ is the set of nodes in (live-edge graph) $L$ that can be reached from $S$.
\end{itemize}

Now we are ready to look at Lemma 2 of~\cite{sun2023scalable}:
\begin{align*}
    \rho_S(A)&=n^-\cdot \mathbb{E}[\mathbb{I}\{A \cap VE (P^S_L)\neq \emptyset\}]\\
    &=\sigma^-(S)\cdot \mathbb{E}[\mathbb{I}\{A \cap VE (P_L)\neq \emptyset\} | S\cap VE(P_L)\neq \emptyset].
\end{align*}
Unfortunately, it seems that using $VE(X)$ leads to a mistake, as the condition $S\cap VE(P_L)\neq \emptyset$ is always false. Here we directly show a corrected version of it:
\begin{align}
    \rho_S(A)&=n^-\cdot \mathbb{E}[\mathbb{I}\{A \cap P^S_L\neq \emptyset\}]\label{equ:advim-lemma-correct1}\\
    &=\sigma^-(S)\cdot \mathbb{E}[\mathbb{I}\{A \cap P_L\neq \emptyset\} | S\cap P_L\neq \emptyset].\label{equ:advim-lemma-correct2}
\end{align}
Both Eq.~\eqref{equ:advim-lemma-correct1} and Eq.~\eqref{equ:advim-lemma-correct2} are correct. Each of them is utilized depending on the RR path generation strategy.

To explain Eq.~\eqref{equ:advim-lemma-correct1}, when we generate a collection (let's say $\R$) that contains multiple `relevant' RR paths $P^S_L$ as defined above, we can use the coverage of $A$ w.r.t. $\R$ as an estimator of $\rho_S(A)$. On the other hand, to explain Eq.~\eqref{equ:advim-lemma-correct2}, the original work uses a different generation method of a `relevant' RR paths $P^S_L$: they repeatedly generate $P_L$, whenever $P_L\cap S=\emptyset$, they generate a new one, until $P_L\cap S\neq\emptyset$ and then let $P^S_L=P_L$. By doing this, they avoid the case where $P^S_L=\emptyset$ and the probability of $\mathbb{I}\{A \cap P^S_L\neq \emptyset\}$ becomes $\mathbb{E}[\mathbb{I}\{A \cap P_L\neq \emptyset\} | S\cap P_L\neq \emptyset]$, which is in Eq.~\eqref{equ:advim-lemma-correct2}.

\stitle{Our modified definition}
If using the original definition of $\rho_S(A)$ and their RR path generation strategy to obtain the value of $\rho_S(A)$, we should multiply the factor $\sigma^-(S)$ by the coverage result, as stated in Eq.~\eqref{equ:advim-lemma-correct2}. But as we know, $\sigma^-(S)$ is difficult to obtain. Therefore, for now, our approach is to modify the definition of $\rho_S(A)$ by scaling a factor of $\frac{n^-}{\sigma^-(S)}$. If this approach is not very convincing, we can revert to the original definition, in which case the value $\kappa$ in our paper, as in Eq.~\eqref{eq:general-spread}, will be equal to $\sigma^-(S)$. Note that the only place where we really need to know $\kappa$ is in Eq.~\eqref{equ:theta_max}, but we can also use the fact $\kappa=\sigma^-(S)\leq n^-$ to avoid computing it.

\stitle{Proofs}
To prove Eq.~\eqref{equ:advim-lemma-correct1}, by the definition of $\rho_S(A)$ we have
\begin{align}
    &\rho_S(A)=\mathbb{E}\left[\left|\left\{v\in V\backslash S:v\in \Gamma(L, S) \text{~and~} v\not\in \Gamma(L\backslash A, S)\right\}\right|\right]\notag\\
    &=n^-\cdot\mathbb{E}_{v\text{~is selected uniformly from~}V\backslash S}\left[\mathbb{I}\left\{v\in \Gamma(L, S) \text{~and~} v\not\in \Gamma(L\backslash A, S)\right\}\right]\notag\\
    &=n^-\cdot\Pr\left\{A\cap P^S_L \neq\emptyset\right\}\label{equ:advim-lemma-correct3},
\end{align}
which shows that Eq.~\eqref{equ:advim-lemma-correct1} holds. To further deducting Eq.~\eqref{equ:advim-lemma-correct2}, we recall that $P^S_L=\emptyset$ if $P_L\cap S=\emptyset$ and $P^S_L=P_L$ if $P_L\cap S\neq\emptyset$. Hence, we have
\begin{align}
    \text{Eq.}~\eqref{equ:advim-lemma-correct3}&=n^-\cdot\left(\Pr\left\{A\cap P_L \neq\emptyset | S\cap P_L \neq\emptyset\right\}\cdot\Pr\left\{S\cap P_L \neq\emptyset\right\}\right).\label{equ:advim-lemma-correct4}
\end{align}
On the other hand, we can derive that
\begin{align*}
    &n^-\cdot\Pr\left\{S\cap P_L \neq\emptyset\right\}=n^-\cdot\frac{\sum_{v\in V\backslash S}\Pr\{v\in \Gamma(L, S)\}}{n^-}\\
    &=\sum_{v\in V\backslash S}\Pr\{v\text{ is influenced by }S\}=\sigma^-(S).
\end{align*}
Substituting the above to Eq.~\eqref{equ:advim-lemma-correct4}, and then we obtain the result in Eq.~\eqref{equ:advim-lemma-correct2}.

% \subsection{Feasibility of using our approach}

% \noindent \textit{Full definition of \prm in ~\cite{liao2023popularity}.} The eventual solvable PRM definition is to maximize the surrogate objective, $\sigma_{PRM}(\cdot)$, under the constraint $\M_{PRM}$ mentioned above. Based on their proposed \textsf{PA-IC} model, given three input parameters $d^n_0, d^p_0, z$, the surrogate objective is defined as $$\sigma_{PRM}(S_1,\dots, S_T)=\sum_{t=1}^T \frac{1}{d^n_0+d^p_0+t\cdot z}\cdot \rho_G(S_t),$$ where $\rho_G(S_t)$ is the spread of $S_t$ in the \ic model. Abstractly speaking, $\rho_G(S_t)$ is the \ic part of \textsf{PA-IC}, and $d^n_0, d^p_0, z$ forms the \textsf{PA} part of \textsf{PA-IC}.

% \textit{Claim.} The \prm problem can be solved by our proposed algorithms \cseedselect and \ouralgo.

% To show the applicability of our solution, we need to verify two aspects: the existence of a general matroid constraint $\M_{PRM}$ (which we have shown previously), and the feasibility of generating RR sets as an unbiased estimator of the objective function $\sigma_{PRM}(\cdot)$. To this end, we denote $\alpha_t=\frac{1}{d^n_0+d^p_0+t\cdot z}$, thus we can rewrite $\sigma_{PRM}(\cdot)$ as $\sigma_{PRM}(S_1,\dots, S_T)=\sum_{t=1}^T \alpha_t \cdot \rho_G(S_t)$, which is reduced to the same form as the objective function of \rim in Section~\ref{sec:imgm-instance}.
% Therefore, we can use the same method as in \rim to solve \prm, by generating many RR sets using \ouralgo (with the same method of sampling one RR set) and maximizing the coverage using \cseedselect.


% \section{An Informal Note of \rim}

% The revenue maximization problem proposed in~\cite{han2021efficient} (dubbed as O-\rim) has additional inputs and constraints than our \rim problem: for each campaign $i\in[T]$ there is a budget $B_i>0$; for each user $v_j\in V$, there is a cost $c_i(v_j)$ of selecting $v_j$ for campaign $i$. The additional constraint in O-\rim than ours is: for each $i\in[T]$, it should be satisfied that $\alpha_i\cdot \rho_G(S_i)+\sum_{v_j\in S_i}c_i(v_j)\leq B_i$. Their approach also consists of an element selection algorithm and an RR set generation algorithm. The element selection algorithm \textsf{RM\_with\_Oracle} is shown in Algorithm 5 in Figure~\ref{fig:rm-algs-screenshot}. For convenience, some notations they used are listed below. \textit{We will use their notation in the following parts. In addition, given that Algorithms 1-2 have the same name as those in our paper, we use \textsf{Greedy-O} and \textsf{ThresholdGreedy-O} to represent Algorithms 1 and 2, respectively.}

% \begin{itemize}
%     \item $h$ equals the number of campaigns, \ie $T$ in \rim.
%     \item $c_i(v)$ is the cost of selecting a node $v\in V$ to campaign $i$, which is given as input;
%     \item $\pi_i(S_i)$ equals $\alpha_i\cdot \rho_G(S_i)$ in our \rim problem. That is, the sum of $\pi_i(S_i)$ for all $i$ equals the objective function in \rim;
%     \item $\zeta_i(u|S_i) = \frac{\pi_i(u|S_i)}{c_i(u)+\pi_i(u|S_i)}$;
%     \item $B_i$ the budget for campaign $i$, which is given as input;
%     \item $\gamma_{max}$ in Algorithm 4 euqals $\max\{B_j, \zeta_j(v|\emptyset):v\in V, j\in [h]\}$.
% \end{itemize}

% \begin{figure}[h]
%     \centering
%     \includegraphics[width=1.0\linewidth]{fig/Screenshot-rm.png}
%     \caption{The element selection algorithm in~\cite{han2021efficient}.}
%     \label{fig:rm-algs-screenshot}
% \end{figure}

% \textit{Claim.} When setting $c_i(v)=1$ for all $i\in [h],v\in V$ and $B_i=+\infty$ for all $i\in [h]$ in O-\rim, the problem is reduced to our \rim problem. In this case, \textsf{RM\_with\_Oracle} is essentially equal to \mgreedy with any given $\tau\in(0,1)$.

% The equivalence of \textsf{RM\_with\_Oracle} and \mgreedy can be broken down into the following two lemmas.

% \begin{lemma}\label{lem:alg1-equal}
%     When $h=1$, \textsf{Greedy-O}($V, 1$) always returns $S^*_1=V$, thus it is essentially equal to \mgreedy.
% \end{lemma}

% \begin{lemma}\label{lem:alg4-equal}
%     When $h=2$, for $b_{min}=1,2$ and all $\tau\in(0,1)$, the output $\vec{S}^*$ of \textsf{Search}($\tau, b_{min}$) is essentially equal to \mgreedy.
% \end{lemma}

% \begin{proof}[Proof of Lemma~\ref{lem:alg1-equal}]
%     In line 1 of \textsf{Greedy-O}($V, 1$), the input set $U=V$ does not change since the condition $c_1(v)+\pi_1(\{v\})>B_1$ will never be satisfied. In line 4, \textsf{Greedy-O} selects a node $u\in U$ and then assigns $U$ to $U-\{u\}$; $u$ is then definitely added into $S_1$ in line 5, because the \texttt{if} condition will always be true. In addition, $D_i$ is always empty since line 6 will never be executed.
%     The selection of $u$ into $S_1$ in lines 4-5 repeats until $U=\emptyset$, resulting in $S^*_1=S_1=V$ in line 7.
% \end{proof}

% \begin{proof}[Proof of Lemma~\ref{lem:alg4-equal}]
%     We first propose the following lemma.
%     \begin{lemma}\label{lem:alg2-equal}
%         For any $\gamma>0$, \textsf{ThresholdGreedy-O} returns a solution set $\vec{S}^*$ which is always equal to that of \mgreedy and a value $b$ which is always $0$.
%     \end{lemma}
%     Given that the solution $\vec{T}$ returned by \textsf{ThresholdGreedy-O} in line 4 is always equal to that of \mgreedy, the set of solutions $\mathcal{Q}$ is then filled by many identical solution sets. Lines 5-7 adjust the values of $\gamma_1,\gamma_2$ (note that $b_1,b_2$ will always be $0$ due to Lemma~\ref{lem:alg2-equal}), which will make the \texttt{repeat} loop eventually terminate but will not affect the values in $\mathcal{Q}$. (w.l.o.g. we can let $B_i\forall i$ be a sufficiently large value so $\gamma_2$ and $\gamma_{max}$ defined in line 1 of will be large but not infinite. ) Notably, the parameter $\tau$ only determines the value of $\gamma_2$. Consequently, line 9 chooses a solution in $\mathcal{Q}$ as the returned $\vec{S}^*$,  equal to that of \mgreedy.
% \end{proof}.

% \begin{proof}[Proof of Lemma~\ref{lem:alg2-equal}]
% For \textsf{ThresholdGreedy-O} in Algorithm 2, line 1 initializes $M\gets V\times [h]$ as $c_j(v)+\pi_j(v)\leq B_j$ is always true. Line 2 initializes $S_j\gets\emptyset$ for all $j\in[h]$. In the \texttt{while} loop, line 4 selects a pair $(u, i)$ in $M$, containing a user $u\in V$ and a campaign $i\in [h]$  with the largest marginal gain $\pi_i(u|S_i)$. This operation is equivalent to \mgreedy which chooses the one with the largest marginal gain w.r.t. the objective function.
% Regarding line 5, both $\zeta_i(u|S_i\cup D_i)<\gamma/B_i$ and $D_i\neq \emptyset$ are always false regardless of any value of $\gamma$, so they do not cause any skip of the loop. ( The former is due to $B_i=+\infty$ and the second is because $D_i$ will be always empty, as we will show later.) Subsequently, line 6 indicates that if the selected user $u$ has been already included in $S_1,\dots, S_j$, then the selection is invalid and needs to be skipped. Notably, this is equal to adhering to the matroid constraint of \rim in \mgreedy. If $u$ has not been selected yet, in line 7, $u$ is definitely added to $S_i$, and line 8 will never be executed, thus $D_i$, $I$ will always be empty. This further replies that lines 9-11 will never be executed, thus $A_i$ will always be empty. Given that the element selection process above is the same as \mgreedy, in line 11, $\vec{S}'$ will be identical to the return solution of \mgreedy, with each $S'_j$ indicating the seed set for campaign $j$. Next, line 12 assigns $\vec{S}^*\gets\mathsf{Fill}(\vec{S}')$, where $\mathsf{Fill}(\vec{S}')$ adds some elements into $\vec{S}'$ if the matroid constraint is still satisfied and returns the new $\vec{S}'$. However, $\vec{S}'$ in line 11 has already reached the largest cardinality, \ie $\vec{S}'$ forms a base of the matroid, thus $\mathsf{Fill}(\vec{S}')$ will not add any nodes and will let $\vec{S}^*\gets\vec{S}'$, which completes the proof.
% \end{proof}
